# Supplementary material for: Mixing Modes: Active and Passive Integration of Speech, Text, and Visualization for Communicating Data Uncertainty
Source: arXiv:2404.08623 source file (2024-04-12)
Supplement: Supplementary file 1 [file appendix.tex]

\section{Experiment 1 Model Summary Table}
\label{section:appendix_E1}

In this appendix, we provide a summary overview of the statistical models and tests used to examine the relationship between three modes: speech, text, and visualization in Experiment 1. These results provide context and further detail to the results reported in Section \ref{section:e1e2_analysis} and \ref{section:e1_results}.

In this table, we display the results for a generalized linear mixed effects model predicting the binary likelihood to salt,  a $\chi^2$ test on decision rationality, a linear mixed effects model on confidence ratings, and a linear model on trust in the forecast overall. Further details on these models (e.g., stepwise regression tables) are available in supplemental materials).

\begin{table}[ht]

\caption{Summary test statistics for Experiment 1 models and $\chi^2$ tests. Reference Level for precision = concrete. Reference levels for mode vary in order to present the most informative pairwise differences. The model summaries do not include the full results of the model, just the hypothesis-relevant variables. Full model details are available in the supplemental materials. Rows highlighted in purple are significant findings.}
\label{tab:e1_stats}
\begin{tabular}{|l|l|l|l|l|}
\hline
\multicolumn{5}{|l|}{\cellcolor[HTML]{C0C0C0}\textbf{Experiment 1}} \\
\hline
\multicolumn{5}{|l|}{\cellcolor[HTML]{EFEFEF}\textbf{Crossover Temperature: Concrete Speech Referent}} \\
\hline
\textbf{Variable} & \textbf{$\beta$} & \textbf{SE} & \textbf{z value} & \textbf{p value} \\ \hline
Mode Text &  -0.287 & 0.664 & -0.431 & 0.666 \\
Mode Visualization  & -0.275 & 0.679 & -0.405 & 0.686 \\
Precision Fuzzy & -1.27 & 0.668 & -1.90 & 0.057 \\
Mode Text * Precision Fuzzy & 1.59 & 0.894 & 1.78 & 0.075 \\
\cellcolor[HTML]{D5D0E6}Mode Visualization * Precision Fuzzy & \cellcolor[HTML]{D5D0E6}1.89 & \cellcolor[HTML]{D5D0E6}0.880 & \cellcolor[HTML]{D5D0E6}2.15 & \cellcolor[HTML]{D5D0E6}0.032 \\
\hline
\multicolumn{5}{|l|}{\cellcolor[HTML]{EFEFEF}\textbf{Decision Rationality}} \\
\hline
\textbf{Comparison} & \textbf{$\chi^2$} & \textbf{df} & \multicolumn{2}{l|}{\textbf{p value}} \\ \hline
Precision & 1.16 & 2 & \multicolumn{2}{l|}{0.559} \\
\cellcolor[HTML]{D5D0E6}Mode & \cellcolor[HTML]{D5D0E6}30.1 & \cellcolor[HTML]{D5D0E6}4 & \multicolumn{2}{l|}{\cellcolor[HTML]{D5D0E6}$<$ 0.01} \\
\hline
\multicolumn{5}{|l|}{\cellcolor[HTML]{EFEFEF}\textbf{Decision Confidence: Concrete Visualization Referent}} \\
\hline
\textbf{Variable} & \textbf{$\beta$} & \textbf{SE} & \textbf{z value} & \textbf{p value} \\ \hline
Mode Text & -5.30 & 2.77 & -1.92 & 0.058 \\
Mode Speech  & -5.29 & 3.02 & -1.75 & 0.083\\
Precision Fuzzy & 0.672 & 2.63 & 0.256 & 0.799 \\
Modey Text * Precision Fuzzy & 1.26 & 3.80 & 0.330 & 0.742 \\
Mode Speech * Precision Fuzzy & 3.78 & 3.91 & 0.967 & 0.336 \\
\hline
\multicolumn{5}{|l|}{\cellcolor[HTML]{EFEFEF}\textbf{Overall Trust: Speech Referent}} \\
\hline
\textbf{Variable} & \textbf{$\beta$} & \textbf{SE} & \textbf{z value} & \textbf{p value} \\ \hline
\cellcolor[HTML]{D5D0E6}Mode Text & \cellcolor[HTML]{D5D0E6}-1.33 & \cellcolor[HTML]{D5D0E6}0.386 & \cellcolor[HTML]{D5D0E6}-3.443 & \cellcolor[HTML]{D5D0E6}$<$ 0.01 \\
\cellcolor[HTML]{D5D0E6}Mode Visualization & \cellcolor[HTML]{D5D0E6}-0.990 & \cellcolor[HTML]{D5D0E6}0.392 & \cellcolor[HTML]{D5D0E6}-2.53 & \cellcolor[HTML]{D5D0E6}0.013 \\
\hline
\end{tabular}
\end{table}

\section{Pilot Image}
\label{section:appendix_pilot}

The following image was shown to pilot participants in Experiment 2 as an explanation for fuzzy and concrete concepts. Note that the illustration does not include any speech, text, or visualization stimuli examples to prevent priming pilot participants with a particular data representation of a concrete and fuzzy concept.

\begin{figure}[ht]
  \includegraphics[width=0.5\linewidth]{figures/fuzzy scale.pdf}
    \caption{Definitions and examples for ``Concrete'' and ``Fuzzy'', adapted from Setlur \& Cogley \cite{setlur2022functional}. Concrete representations provide a clearer or more tangible representation than fuzzy representations, which tend to be more subjective or ambiguous. }
    \Description{Scale depicting an arrow ranging from ``More Concrete'' to ``More Fuzzy''. The fuzzy end of the arrow lists adjectives, ``safe, best, healthy,'' with the label ``Subjective adjectives.''. In the middle, adjectives are ``cheap, low, high, expensive,'' with the label ``Graded adjectives on numerical quantities''. The concrete end of the arrow lists ``tallest, cheapest, and most expensive,'' with the label ``Superlatives on numerical quantities.''}
    \label{fig:concrete_fuzzy}
\end{figure}

\section{Experiment 2 Model Summary Tables}
\label{section:appendix_E2}

In this appendix, we provide a summary overview of the statistical models and tests used to examine the relationship between five levels of precision: most concrete, somewhat concrete, mixed, somewhat fuzzy, and most fuzzy. These results provide context and further detail to the results reported in Section \ref{section:e1e2_analysis} and \ref{section:e2_results}.

For each mode, we present tables that display the results for a generalized linear mixed effects model predicting the binary likelihood to salt,  a $\chi^2$ test on decision rationality, a linear mixed effects model on confidence ratings, and a linear model on trust in the forecast overall. The model summaries do not include the full results of the model, just the hypothesis-relevant variables. Full details on models (e.g., stepwise regression tables) are available in supplemental materials). 

\begin{table}[h]

\caption{Summary of statistical results for Speech conditions in Experiment 2 (models and $\chi^2$). Reference levels for precision is most fuzzy.}
\label{tab:e2_stats2a}
\begin{tabular}{|l|l|l|l|l|}
\hline
\multicolumn{5}{|l|}{\cellcolor[HTML]{C0C0C0}\textbf{Experiment 2: Speech Forecasts}} \\
\hline
\multicolumn{5}{|l|}{\cellcolor[HTML]{EFEFEF}\textbf{Crossover Temperature: Baseline Model}} \\
\hline
\textbf{Variable} & \textbf{$\beta$} & \textbf{SE} & \textbf{z value} & \textbf{p value} \\ \hline
Difference From Optimal Temperature &  -2.97 & 0.187 & -15.89 & $<$ 0.001 \\
\hline
\multicolumn{5}{|l|}{\cellcolor[HTML]{EFEFEF}\textbf{Decision Rationality}} \\
\hline
\textbf{Comparison} & \textbf{$\chi^2$} & \textbf{df} & \multicolumn{2}{l|}{\textbf{p value}} \\ \hline
Precision & 3.17 & 8 & \multicolumn{2}{l|}{0.923} \\
\hline
\multicolumn{5}{|l|}{\cellcolor[HTML]{EFEFEF}\textbf{Decision Confidence: Most Fuzzy Referent}} \\
\hline
\textbf{Variable} & \textbf{$\beta$} & \textbf{SE} & \textbf{z value} & \textbf{p value} \\ \hline
Most Concrete & 3.23 & 2.58 & 1.25 & 0.213 \\
Somewhat Concrete  & 3.62 & 2.62 & 1.38 & 0.170 \\
Mixed & 2.22 & 2.68 & 0.827 & 0.410 \\
Somewhat Fuzzy & 1.68 & 2.68 & 0.628 & 0.53 \\
\hline
\multicolumn{5}{|l|}{\cellcolor[HTML]{EFEFEF}\textbf{Overall Trust: Baseline Model}} \\
\hline
\textbf{Variable} & \textbf{$\beta$} & \textbf{SE} & \textbf{z value} & \textbf{p value} \\ \hline
Decision Rationality [1,0] &  1.27 & 1.25 & 1.02 & 0.311 \\
\hline
\end{tabular}
\end{table}

\begin{table}[h]

\caption{Summary of statistical results for Text conditions in Experiment 2 (models and $\chi^2$ tests). Reference levels vary in order to present the most informative pairwise differences.}
\label{tab:e2_stats2b}
\begin{tabular}{|l|l|l|l|l|}
\hline
\multicolumn{5}{|l|}{\cellcolor[HTML]{C0C0C0}\textbf{Experiment 2: Text Forecasts}} \\
\hline
\multicolumn{5}{|l|}{\cellcolor[HTML]{EFEFEF}\textbf{Crossover Temperature: Most Fuzzy Referent}} \\
\hline
\textbf{Variable} & \textbf{$\beta$} & \textbf{SE} & \textbf{z value} & \textbf{p value} \\ \hline
Most Concrete & -0.304 & 0.376 & -0.809 & 0.418 \\
Somewhat Concrete & -0.068 & 0.355 & -0.187 & 0.851 \\
Mixed & 0.062 & 0.355 & 0.175 & 0.861 \\
Somewhat Fuzzy & -0.185 & 0.355 & -0.522 & 0.602 \\
\hline
\multicolumn{5}{|l|}{\cellcolor[HTML]{EFEFEF}\textbf{Decision Rationality}} \\
\hline
\textbf{Comparison} & \textbf{$\chi^2$} & \textbf{df} & \multicolumn{2}{l|}{\textbf{p value}} \\ \hline
Precision & 3.58 & 8 & \multicolumn{2}{l|}{0.893} \\
\hline
\multicolumn{5}{|l|}{\cellcolor[HTML]{EFEFEF}\textbf{Decision Confidence: Most Concrete Referent}} \\
\hline
\textbf{Variable} & \textbf{$\beta$} & \textbf{SE} & \textbf{z value} & \textbf{p value} \\ \hline
\cellcolor[HTML]{D5D0E6}Somewhat Concrete  & \cellcolor[HTML]{D5D0E6}-5.19 & \cellcolor[HTML]{D5D0E6}2.57 & \cellcolor[HTML]{D5D0E6}-2.02 & \cellcolor[HTML]{D5D0E6}0.045 \\
Mixed & -1.96 & 2.61 & -0.752 & 0.454 \\
\cellcolor[HTML]{D5D0E6}Somewhat Fuzzy & \cellcolor[HTML]{D5D0E6}-5.15 & \cellcolor[HTML]{D5D0E6}2.57 & \cellcolor[HTML]{D5D0E6}-2.01 & \cellcolor[HTML]{D5D0E6}0.047 \\
Most Fuzzy & -4.03 & 2.61 & -1.54 & 0.1256 \\
\hline
\multicolumn{5}{|l|}{\cellcolor[HTML]{EFEFEF}\textbf{Overall Trust: Most Fuzzy Referent}} \\
\hline
\textbf{Variable} & \textbf{$\beta$} & \textbf{SE} & \textbf{z value} & \textbf{p value} \\ \hline
\cellcolor[HTML]{D5D0E6}Most Concrete & \cellcolor[HTML]{D5D0E6}1.83 & \cellcolor[HTML]{D5D0E6}0.513 & \cellcolor[HTML]{D5D0E6}3.57 & \cellcolor[HTML]{D5D0E6}0.001 \\
Somewhat Concrete  & 0.756 & 0.494 & 1.53 & 0.129 \\
\cellcolor[HTML]{D5D0E6}Mixed & \cellcolor[HTML]{D5D0E6}1.15 & \cellcolor[HTML]{D5D0E6}0.504 & \cellcolor[HTML]{D5D0E6}2.28 & \cellcolor[HTML]{D5D0E6}0.024 \\
Somewhat Fuzzy & 1.01 & 0.494 & 2.05 & 0.043 \\
\hline
\end{tabular}
\end{table}

\begin{table}[h]

\caption{Summary of statistical results for Visualization conditions in Experiment 2 (models and $\chi^2$ tests). Reference levels vary in order to present the most informative pairwise differences.}
\label{tab:e2_stats2c}
\begin{tabular}{|l|l|l|l|l|}
\hline
\multicolumn{5}{|l|}{\cellcolor[HTML]{C0C0C0}\textbf{Experiment 2: Visualization Forecasts}} \\
\hline
\multicolumn{5}{|l|}{\cellcolor[HTML]{EFEFEF}\textbf{Crossover Temperature: Most Concrete Referent}} \\
\hline
\textbf{Variable} & \textbf{$\beta$} & \textbf{SE} & \textbf{z value} & \textbf{p value} \\ \hline
Somewhat Concrete  & 0.610 &  0.366 & 1.67 & 0.095 \\
Mixed & 0.468 & 0.350 & 1.34 & 0.182 \\
\cellcolor[HTML]{D5D0E6}Somewhat Fuzzy & \cellcolor[HTML]{D5D0E6}1.16 & \cellcolor[HTML]{D5D0E6}0.367 & \cellcolor[HTML]{D5D0E6}3.16 & \cellcolor[HTML]{D5D0E6}0.002 \\
Most Fuzzy & 0.661 & 0.359 & 1.84 & 0.066 \\
\hline
\multicolumn{5}{|l|}{\cellcolor[HTML]{EFEFEF}\textbf{Decision Rationality}} \\
\hline
\textbf{Comparison} & \textbf{$\chi^2$} & \textbf{df} & \multicolumn{2}{l|}{\textbf{p value}} \\ \hline
\cellcolor[HTML]{D5D0E6}Precision & \cellcolor[HTML]{D5D0E6}16.2 & \cellcolor[HTML]{D5D0E6}8 & \multicolumn{2}{l|}{\cellcolor[HTML]{D5D0E6}0.040} \\
\hline
\multicolumn{5}{|l|}{\cellcolor[HTML]{EFEFEF}\textbf{Decision Confidence: Most Fuzzy Referent}} \\
\hline
\textbf{Variable} & \textbf{$\beta$} & \textbf{SE} & \textbf{z value} & \textbf{p value} \\ \hline
Most Concrete & 2.12 & 2.10 & 1.01 & 0.315 \\
Somewhat Concrete  & -0.370 &  2.17 & -0.170 & 0.865 \\
Mixed & -1.23 & 2.08 & -0.591 & 0.555 \\
Somewhat Fuzzy & 1.63 & 2.12 & -0.767 & 0.445 \\
\hline
\multicolumn{5}{|l|}{\cellcolor[HTML]{EFEFEF}\textbf{Overall Trust: Baseline Model}} \\
\hline
\textbf{Variable} & \textbf{$\beta$} & \textbf{SE} & \textbf{z value} & \textbf{p value} \\ \hline
Decision Rationality [1,0] &  3.76 & 1.35 & 0.311 & 0.006\\
\hline
\end{tabular}
\end{table}
